# Supplementary material for: QDFormer: Towards Robust Audiovisual Segmentation in Complex Environments with Quantization-based Semantic Decomposition
Source: arXiv:2310.00132 source file (2024-04-19)
Supplement: Supplementary file 1 [file supp.tex]

\section{More Experiments}

\begin{table}[h]
\centering
\begin{tabular}{cp{1.4cm}
<{\centering}p{1.4cm}<{\centering}} 
\hline
\multirow{2}*{Pvt-v2 \cite{wang2022pvt}} &
Object-M & Sementic\\
\cline{2-3}
~ & $\mathcal{J} \& \mathcal{F}$ & mIoU\\
\hline
AVSBench \cite{zhou2022avs} & 59.3 & 29.8 \\
AVSegFormer \cite{gao2023avsegformer} & 63.8 & 42.0 \\
CATR \cite{li2023catr} &  64.5 & 32.8\\
\rowcolor{verylightgray} Ours & 65.8 & 54.5\\
\hline
\end{tabular}
\caption{Performance with larger backbone.}
\label{tab:larger backbone}
\vspace{-0.8cm}
\end{table}

\paragraph{Larger backbone.}
We demonstrate the performance on AVSBench test set with Pvt-v2 \cite{wang2022pvt} backbone as shown in \cref{tab:larger backbone}. We notice that our method consistently outperforms previous baselines CATR \cite{li2023catr} and AVSegFormer \cite{gao2023avsegformer} on both AVS-Object-Multi and AVS-Semantic datasets. 
% The superior performance demonstrates the effectiveness of the proposed quantization-based semantic decomposition.

\begin{table}[h]
\centering
\begin{tabular}{cp{1.4cm}
<{\centering}p{1.4cm}<{\centering}} 
\hline
\multirow{2}*{frame number} &
Object-M & Sementic\\
\cline{2-3}
~ & $\mathcal{J} \& \mathcal{F}$ & mIoU\\
\hline
3 & 60.9 & 45.4\\
\rowcolor{verylightgray}5 & 61.6 & 46.6\\
7 & - & 46.6 \\
\hline
\end{tabular}
\caption{Ablation on the input frame number.}
\label{tab:Frame number}
\end{table}

\noindent\textbf{Frame number.}
We ablate the influence of input frame number during training. As shown in \cref{tab:Frame number}, we notice a frame number of five achieves the best performance. For the AVS-Object dataset, since the maximum clip length is five, we do not experiment with larger frame number. Please note that the frame number is only fixed during training and the model can accept arbitrary frame numbers during inference.

\begin{table}[h]
\centering
\begin{tabular}{cp{1.4cm}
<{\centering}p{1.4cm}<{\centering}} 
\hline
\multirow{2}*{layer number} &
Object-M & Sementic\\
\cline{2-3}
~ & $\mathcal{J} \& \mathcal{F}$ & mIoU\\
\hline
1 & 61.3 & 45.6 \\
\rowcolor{verylightgray}3 & 61.6 & 46.6\\
5 & 61.0 & 46.0\\
\hline
\end{tabular}
\caption{Ablation on transformer decoder layer number.}
\label{tab:layer}
\end{table}

\noindent\textbf{Transformer decoder layer number.}
We conduct an ablation study on transformer decoder layer numbers in semantic decoders. As shown in \cref{tab:layer}, a transformer decoder layer of 3 achieves the best performance. We notice that even a single-layer transformer decoder for semantic decomposition can lead to a good performance. 

\begin{table}[h]
\centering
\begin{tabular}{cp{1.4cm}
<{\centering}p{1.4cm}<{\centering}} 
\hline
\multirow{2}*{frame resolution} & Sementic\\
\cline{2-2}
~ & mIoU\\
\hline
224$\times$ & 46.6\\
\rowcolor{verylightgray}640$\times$  & 49.2\\
\hline
\end{tabular}
\caption{Ablation on input frame resolution.}
\label{tab:resolution}
\end{table}

\noindent\textbf{Input Resolution.}
The default setting of AVSBench is $224\times 224$ (following the sound source localization convention) for both AVS-Object and AVS-Semantic datasets. While AVS-Semantic actually provides high-resolution (720p) frames. We conduct experiments to ablate the input resolution to facilitate future comparison. Following the semantic segmentation convention, we scale the input frames to the longest side $224$ or $640$. The results are illustrated in \cref{tab:resolution}. We only conduct ablation on AVS-Semantic since the resolution of AVS-Object is low-resolution ($224\times 224$). The results are reported with the ResNet-50 backbone.

\begin{table}[h]
\centering
\scalebox{1}{
\begin{tabular}{ccc}
\hline
Token & Object-M & Sementic\\
\cline{2-3}
Number & $\mathcal{J} \& \mathcal{F}\uparrow$ & mIoU$\uparrow$\\
\hline
1 & 59.7 & 40.2 \\
3 & 61.0 & 43.5 \\
\rowcolor{verylightgray}5 & 61.6 & 46.6 \\
7 & 61.6 & 45.9 \\
9 & 61.2 & 46.3 \\
\hline
\end{tabular}
}
\caption{Ablation on decomposed token number.}
\label{tab:token_number}
\end{table}

\noindent\textbf{Ablation on semantic token number.}
We ablate the semantic token number for the global-ASD and local-ASD in \cref{tab:token_number}. We observe that a token number of 5 yielded the best performance. This can be attributed to the fact that the maximum number of mixed sound sources for the audio-visual dataset is 5.

\begin{table}[h]
\centering
\begin{tabular}{ccc}
\hline
{Codebook } &
Object-M & Sementic\\
\cline{2-3}
Size & $\mathcal{J} \& \mathcal{F}\uparrow$ & mIoU$\uparrow$\\
\hline
1 & 52.7 & 24.8\\
32 & 61.4 & 31.5\\
64 & 60.0 & 43.2 \\
\rowcolor{verylightgray}128 & 61.6 & 46.6\\
256 & 60.6 & 46.1 \\
\hline
\end{tabular}
\caption{Ablation on codebook size.}
\label{tab:codebook_size}
\end{table}

\noindent\textbf{Ablation on codebook size.}
The cardinality of the codebook is essential to our semantic decomposition. Ideally, we aim to constrain the cardinality of the codebook to be close to the semantic category number. We ablate on codebook size from 1 to 256. When the codebook size equals 1, all the decomposed audio tokens are the same, resulting in all the same segmentation results. As shown in \cref{tab:codebook_size}, we notice even a codebook size of 1 achieves 24.8 $\mathrm{mIoU}$ on AVS-Semantic. 
A codebook of size=128 achieves the best performance. Please note that a codebook size slightly larger than the category number, \eg 128, will not hamper the semantic decomposition capability of our method, since 
$128 \ll 70^N$ where $N>1$ is the maximum sound source number, and 70 is the category number.

\begin{figure*}[t]
    \centering
    \scalebox{1}{
    \includegraphics[width=\linewidth]{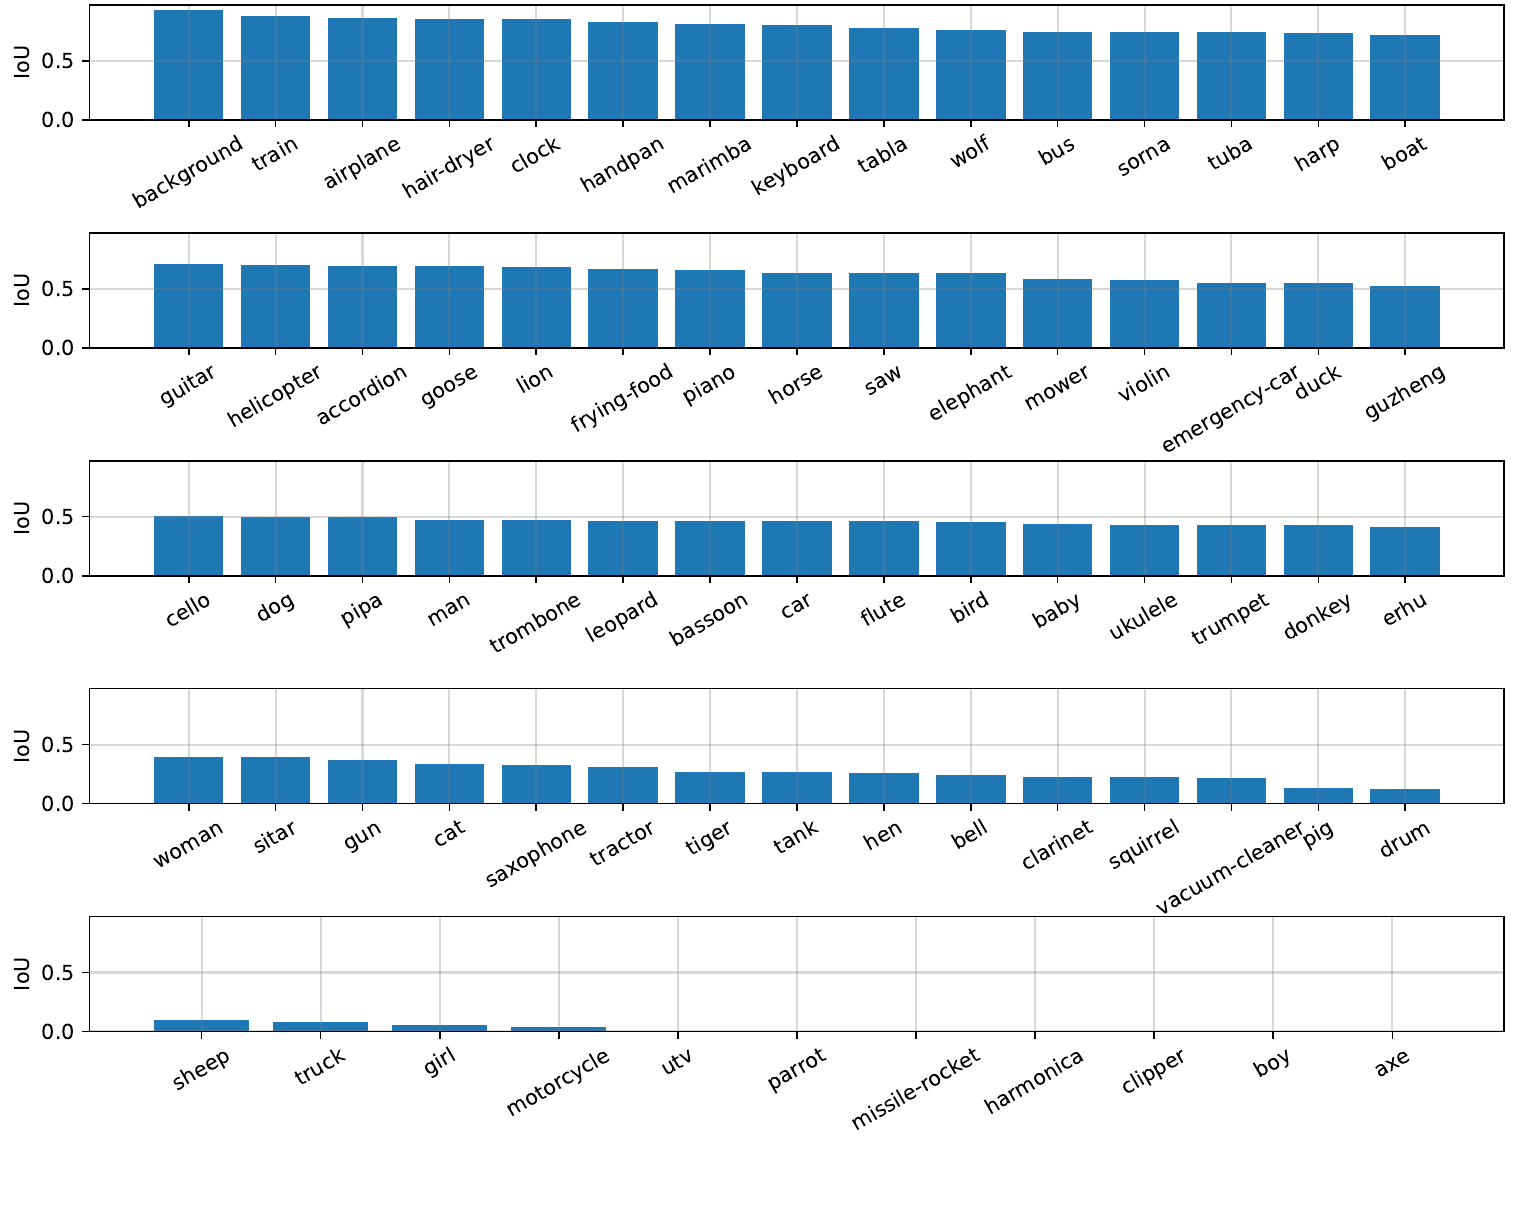}
    }\vspace{-10mm}
    \caption{\textbf{Per-class IOU Analysis.} Our model demonstrates strong audio-guided segmentation capabilities for common head classes, accurately capturing 'background', 'train', 'airplane', 'hair-dryer', and 'clock' with high precision. However, the limited data samples for tail classes like 'utv', 'parrot', 'missile-rocket', 'harmonica', 'clipper', 'boy', and 'ax' due to a long tail distribution adversely affect the model's segmentation performance, hindering accurate identification and delineation of these classes.}
    \label{fig:iou_per_class}
\end{figure*}

\vspace{0.1cm}
\noindent\textbf{Importance of the single-source audio on the semantic decomposition of multi-source audio representation.}

\begin{figure}[h]
    \centering
    \includegraphics[width=\linewidth]{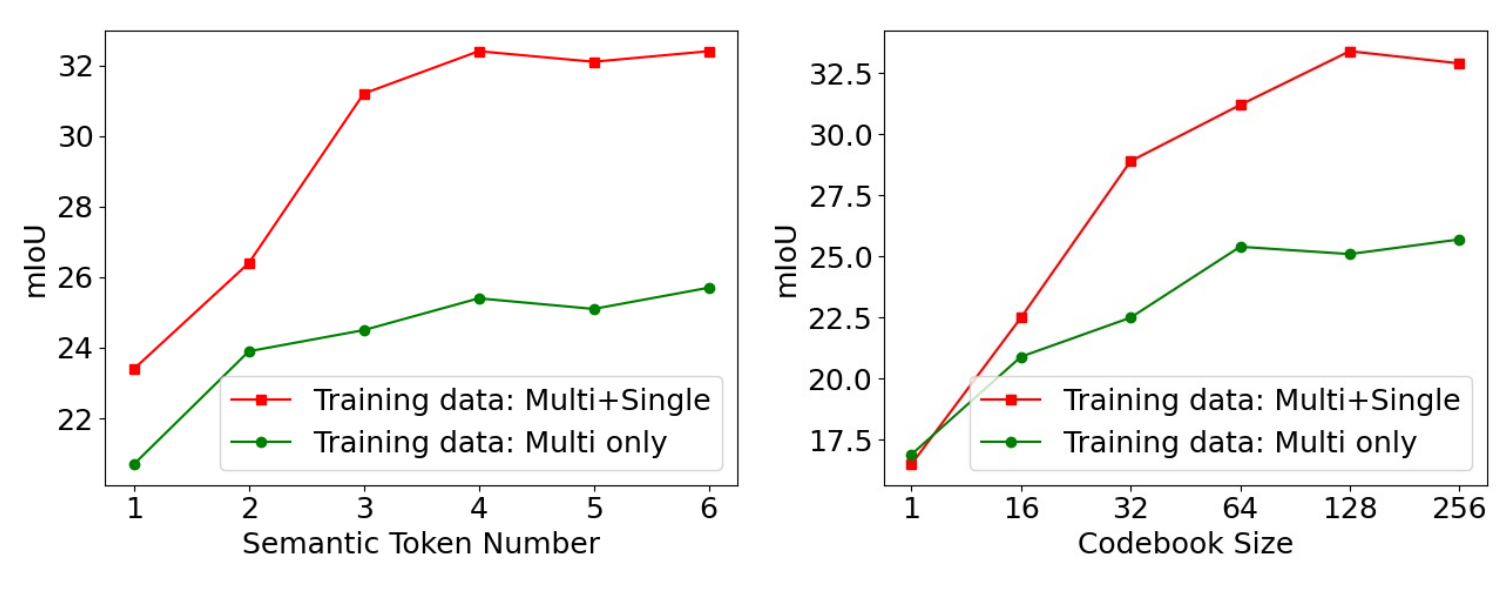}
    \caption{Comparison of training w. and w./o. single-source data.} 
    \label{fig:input type}
\end{figure}

We present empirical evidence that the single-source audio samples significantly contribute to the success of semantic decomposition. 
To demonstrate this, we compare the performance of our model trained on two training sets with the same number of samples: one contains solely multi-source audio samples, and the other contains single- and multi-source audio samples with a ratio of 1:1.
As illustrated in \cref{fig:input type}, the model trained solely on multi-source audio samples exhibits inferior performance compared to the model trained on both types of samples, regardless of the token number and codebook size. 
We conjecture that the single-source samples serve as informative anchors that assist the model in learning the correct distributions of the decomposed simplex spaces for multi-source samples. 
In the absence of single-source samples, the decomposition task could be more difficult due to the absence of such informative anchors.

\noindent\textbf{Per-class IOU analysis.} As is shown in Fig.~\ref{fig:iou_per_class}, we show the per-class iou score on the AVS-Semantic dataset.
Our model demonstrates strong audio-guided segmentation capabilities for common head classes such as 'background', 'train', 'airplane', 'hair-dryer' and 'clock'. These classes are accurately segmented with a high level of precision and reliability. The model effectively distinguishes the 'background' class, providing a solid foundation for identifying and isolating foreground objects. It accurately segments transportation-related classes like 'train', 'airplane', and 'bus' capturing their intricate details and boundaries. Similarly, it excels in segmenting objects such as 'hair-dryer', 'clock' and 'tabla,' effectively separating them from the background. Even for more complex and nuanced classes like 'wolf,' our model demonstrates commendable segmentation performance, accurately delineating the contours and shape of the subject. Overall, our model showcases its ability to segment these common head classes with high accuracy and proficiency, making it a reliable choice for various segmentation tasks.

However, the scarcity of data samples for tail classes like 'utv', 'parrot', 'missile-rocket', 'harmonica', 'clipper', 'boy' and 'ax' in the presence of a long tail distribution can significantly impact the performance of our model, specifically in the task of segmentation. With limited examples to learn from, the model finds it challenging to capture the intricate patterns and unique characteristics associated with these classes. Consequently, the accuracy and reliability of segmentation results for the tail classes may be compromised, leading to suboptimal performance in accurately identifying and delineating these objects or entities of interest.

% \section{More Related Works}
% Audiovisual segmentation also closely relates to video object segmentation (VOS) \cite{yang2018efficient,jain2017fusionseg,cheng2021modular,seong2020kernelized,hu2021learning,cheng2021stcn,seong2021hierarchical,yang2021associating} and video semantic segmentation (VSS) \cite{li2018low,sun2022coarse,zhuang2022semi,hu2020temporally,paul2020efficient}. AVS requires understanding the visual contents and then corresponding them with the audio semantics to segment objects. Specifically, the most closely related task in the video segmentation domain is the referring video object segmentation (RVOS) \cite{botach2021mttr,referformer,urvos} which aims to segment objects in the visual frames given a linguistic expression. For each expression, RVOS only refers to one object while the AVS task permits audio query to refer to multiple objects which makes AVS task more challenging.

\begin{figure*}[t]
    \centering
    \scalebox{1}{
    \includegraphics[width=\linewidth]{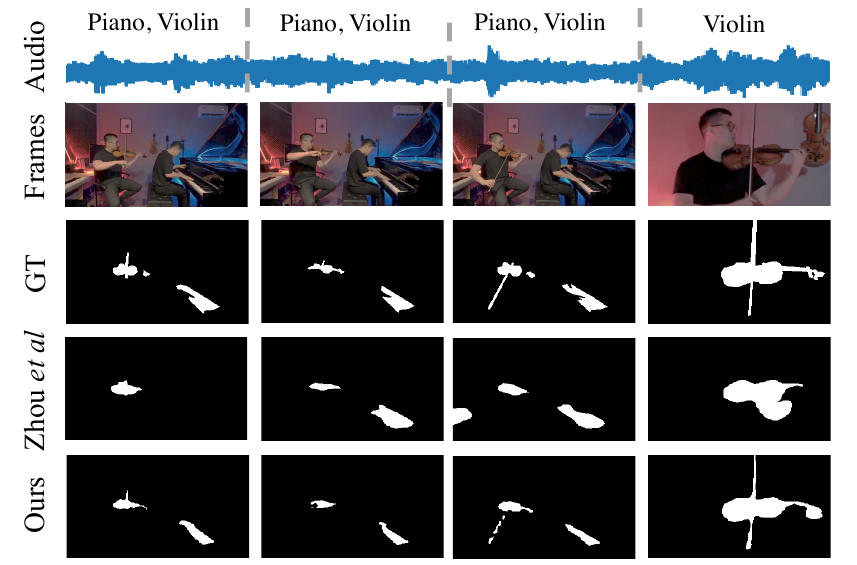}
    }
    \caption{Qualitative comparison to  Zhou \etal$\,$ \cite{zhou2023audio} on AVS-Object. Our method outperforms Zhou et al.'s approach by consistently and accurately segmenting the correct objects throughout the entire video clip, showcasing superior performance and better mask quality. These results emphasize the effectiveness and robustness of our approach in achieving accurate object segmentation in audio-visual scenes. }
    \label{fig:vis_obj}
\end{figure*}

\section{More Visualization \& Video Demo}

\noindent\textbf{More qualitative results on AVS-Object.}  In our study, we provide visualizations of the qualitative results on AVS-Object, as shown in \cref{fig:vis_obj}. We compare our method with the approach proposed by Zhou et al. \cite{zhou2023audio} and observe a notable difference in performance. Specifically, in the third frame of the video clip, the method proposed by Zhou et al. suffers from the false-positive problem, incorrectly segmenting objects. In contrast, our method consistently and accurately segments the correct objects throughout the entire video clip, demonstrating superior performance. Additionally, our method showcases better mask quality, with more precise and detailed segmentation boundaries. These results highlight the effectiveness and robustness of our approach in achieving accurate object segmentation in audio-visual scenes.

\noindent\textbf{More qualitative results on AVS-Semantics.} As is shown in Fig.~\ref{fig:qualitative_1}, Fig.~\ref{fig:qualitative_2},  Fig.~\ref{fig:qualitative_3}  and Fig.~\ref{fig:qualitative_4}, our model exhibits exceptional proficiency in accurately segmenting both multiple and tiny sounding objects, showcasing its versatility and robustness in audio-guided segmentation tasks. Through the implementation of a decomposed and discretized audio representation, our model effectively captures the distinct acoustic characteristics of various objects, enabling precise delineation of multiple simultaneous sound sources. Furthermore, the model demonstrates remarkable capability in capturing the intricate details and nuances of tiny sounding objects, ensuring accurate segmentation outcomes even for the smallest entities.

% \noindent\textbf{Failure case analysis.}  In certain instances, our model encounters failures in achieving high-quality segmentation of objects. As is shown in Fig.~\ref{fig:failure}, while our model can generally differentiate between various sounding objects in the given case, it falls short in accurately delineating the boundary of the piano. The segmentation outcome for the piano exhibits deficiencies, indicating that our model faces challenges in precisely capturing the boundaries and contours of this particular object. We consider that failure can result from the insufficient sample of piano categories in the dataset. By leveraging semantically discrete and decomposed audio features, the model has captured the rough location of the target object. With more image-mask pairs of that category, we consider the performance of the proposed model can be further improved to segment accurate object boundaries. 

\noindent\textbf{Video demo (with audio).} 
We strongly recommend viewing the demo video provided in the supplementary materials, ensuring that you enable audio playback. Watching the video with audio will provide a comprehensive understanding of our audio-visual segmentation application, showcasing how our model utilizes a decomposed and discretized representation to achieve precise audio-visual segmentation results.

\section{More Implementation Details}
We set the $\lambda_{cls}=2$, $\lambda_{L1}=5$, $\lambda_{giou}=2$, $\lambda_{dice}=2$, $\lambda_{focal}=5$, $\lambda_{com}=0.5$ and $\lambda_{quant}=1$ during all training process. A mask confidence threshold of 0.5 and a class confidence threshold of 0.1 is leveraged to filter out low-confident predictions. 
$C_v=C_e=C_q=256$ is utilized. The positional embedding added in the transformers is the standard triangle positional embedding used in \cite{vaswani2017attention}. We set the layer number to three for all the transformers decoders (including local ASD, global ASD and $\mathrm{TrD}_{segm}$ in mask decoder). 

\subsection{Encoders}
\noindent\textbf{Visual encoder.}
We extract frame-level visual features from each frame $I_t$ with a shared backbone. The $T$ extracted features are then fed into the deformable transformer encoder to further conduct temporal aggregation. Let us denote the extracted visual features as $F_v=\{f_t\}^T_{t=1}$, where $f_t \in \mathbb{R}^{C_{v} \times H \times W}$, and $C_v$, $H$, $W$ denote the channel, height, width of the feature. 

\noindent\textbf{Acoustic encoder.} We use VGGish \cite{hershey2017cnn} to extract audio features. Let the extracted audio feature be $F_a\in\mathbb{R}^{C_{a}\times L_{a}}$ where $C_{a}$ is the dimension of acoustic feature space, and $L_{a}$ is the audio clip length. Note that audio and video frames are already synchronized, thus the length of the audio clip is the same as the length of the video clip.

\begin{figure*}[t]
    \centering
    \scalebox{1}{
    \includegraphics[width=\linewidth]{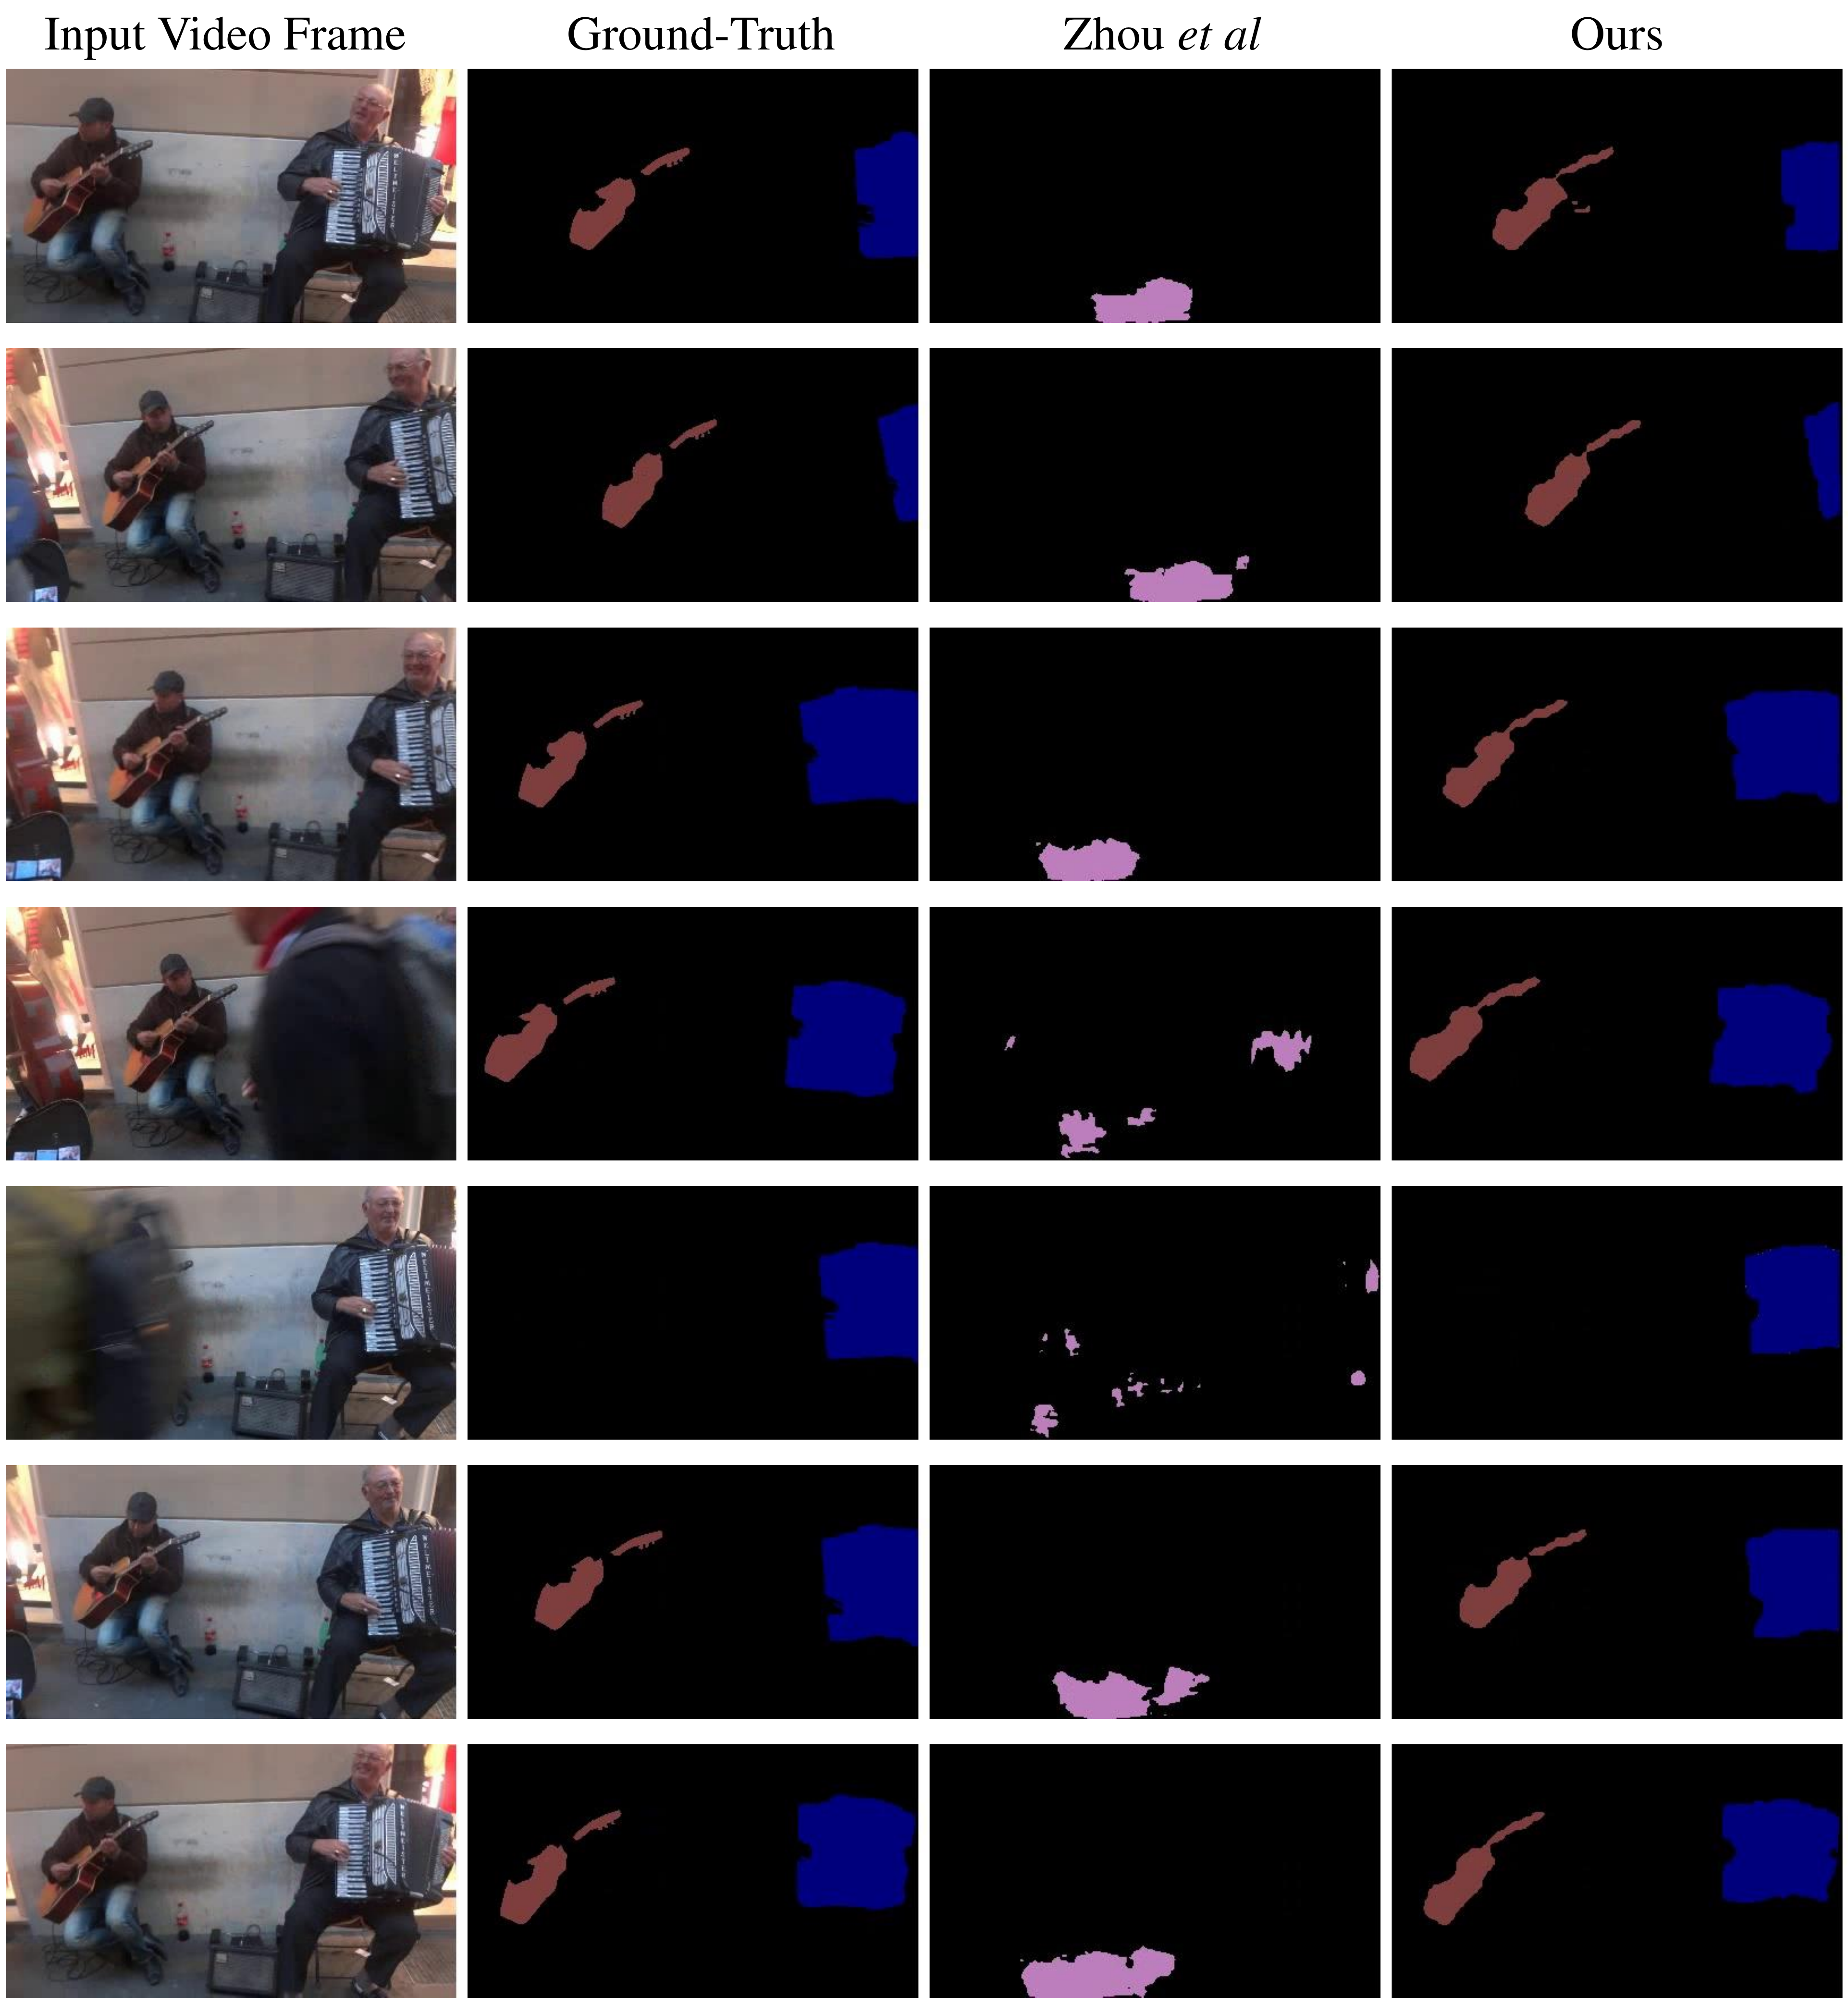}
    }
    \caption{Qualitative comparison to  Zhou \etal$\,$ \cite{zhou2023audio} on AVS-Semantic. Each color represents a semantic category. Our model excels in accurately segmenting \textbf{multiple sounding objects}, showcasing its proficiency in audio-guided segmentation. This success can be attributed to the effective utilization of a decomposed and discretized audio representation, which enables the model to capture and analyze the distinct acoustic features of each object, resulting in precise segmentation outcomes.}
    \label{fig:qualitative_1}
\end{figure*}

\begin{figure*}[t]
    \centering
    \scalebox{1}{
    \includegraphics[width=\linewidth]{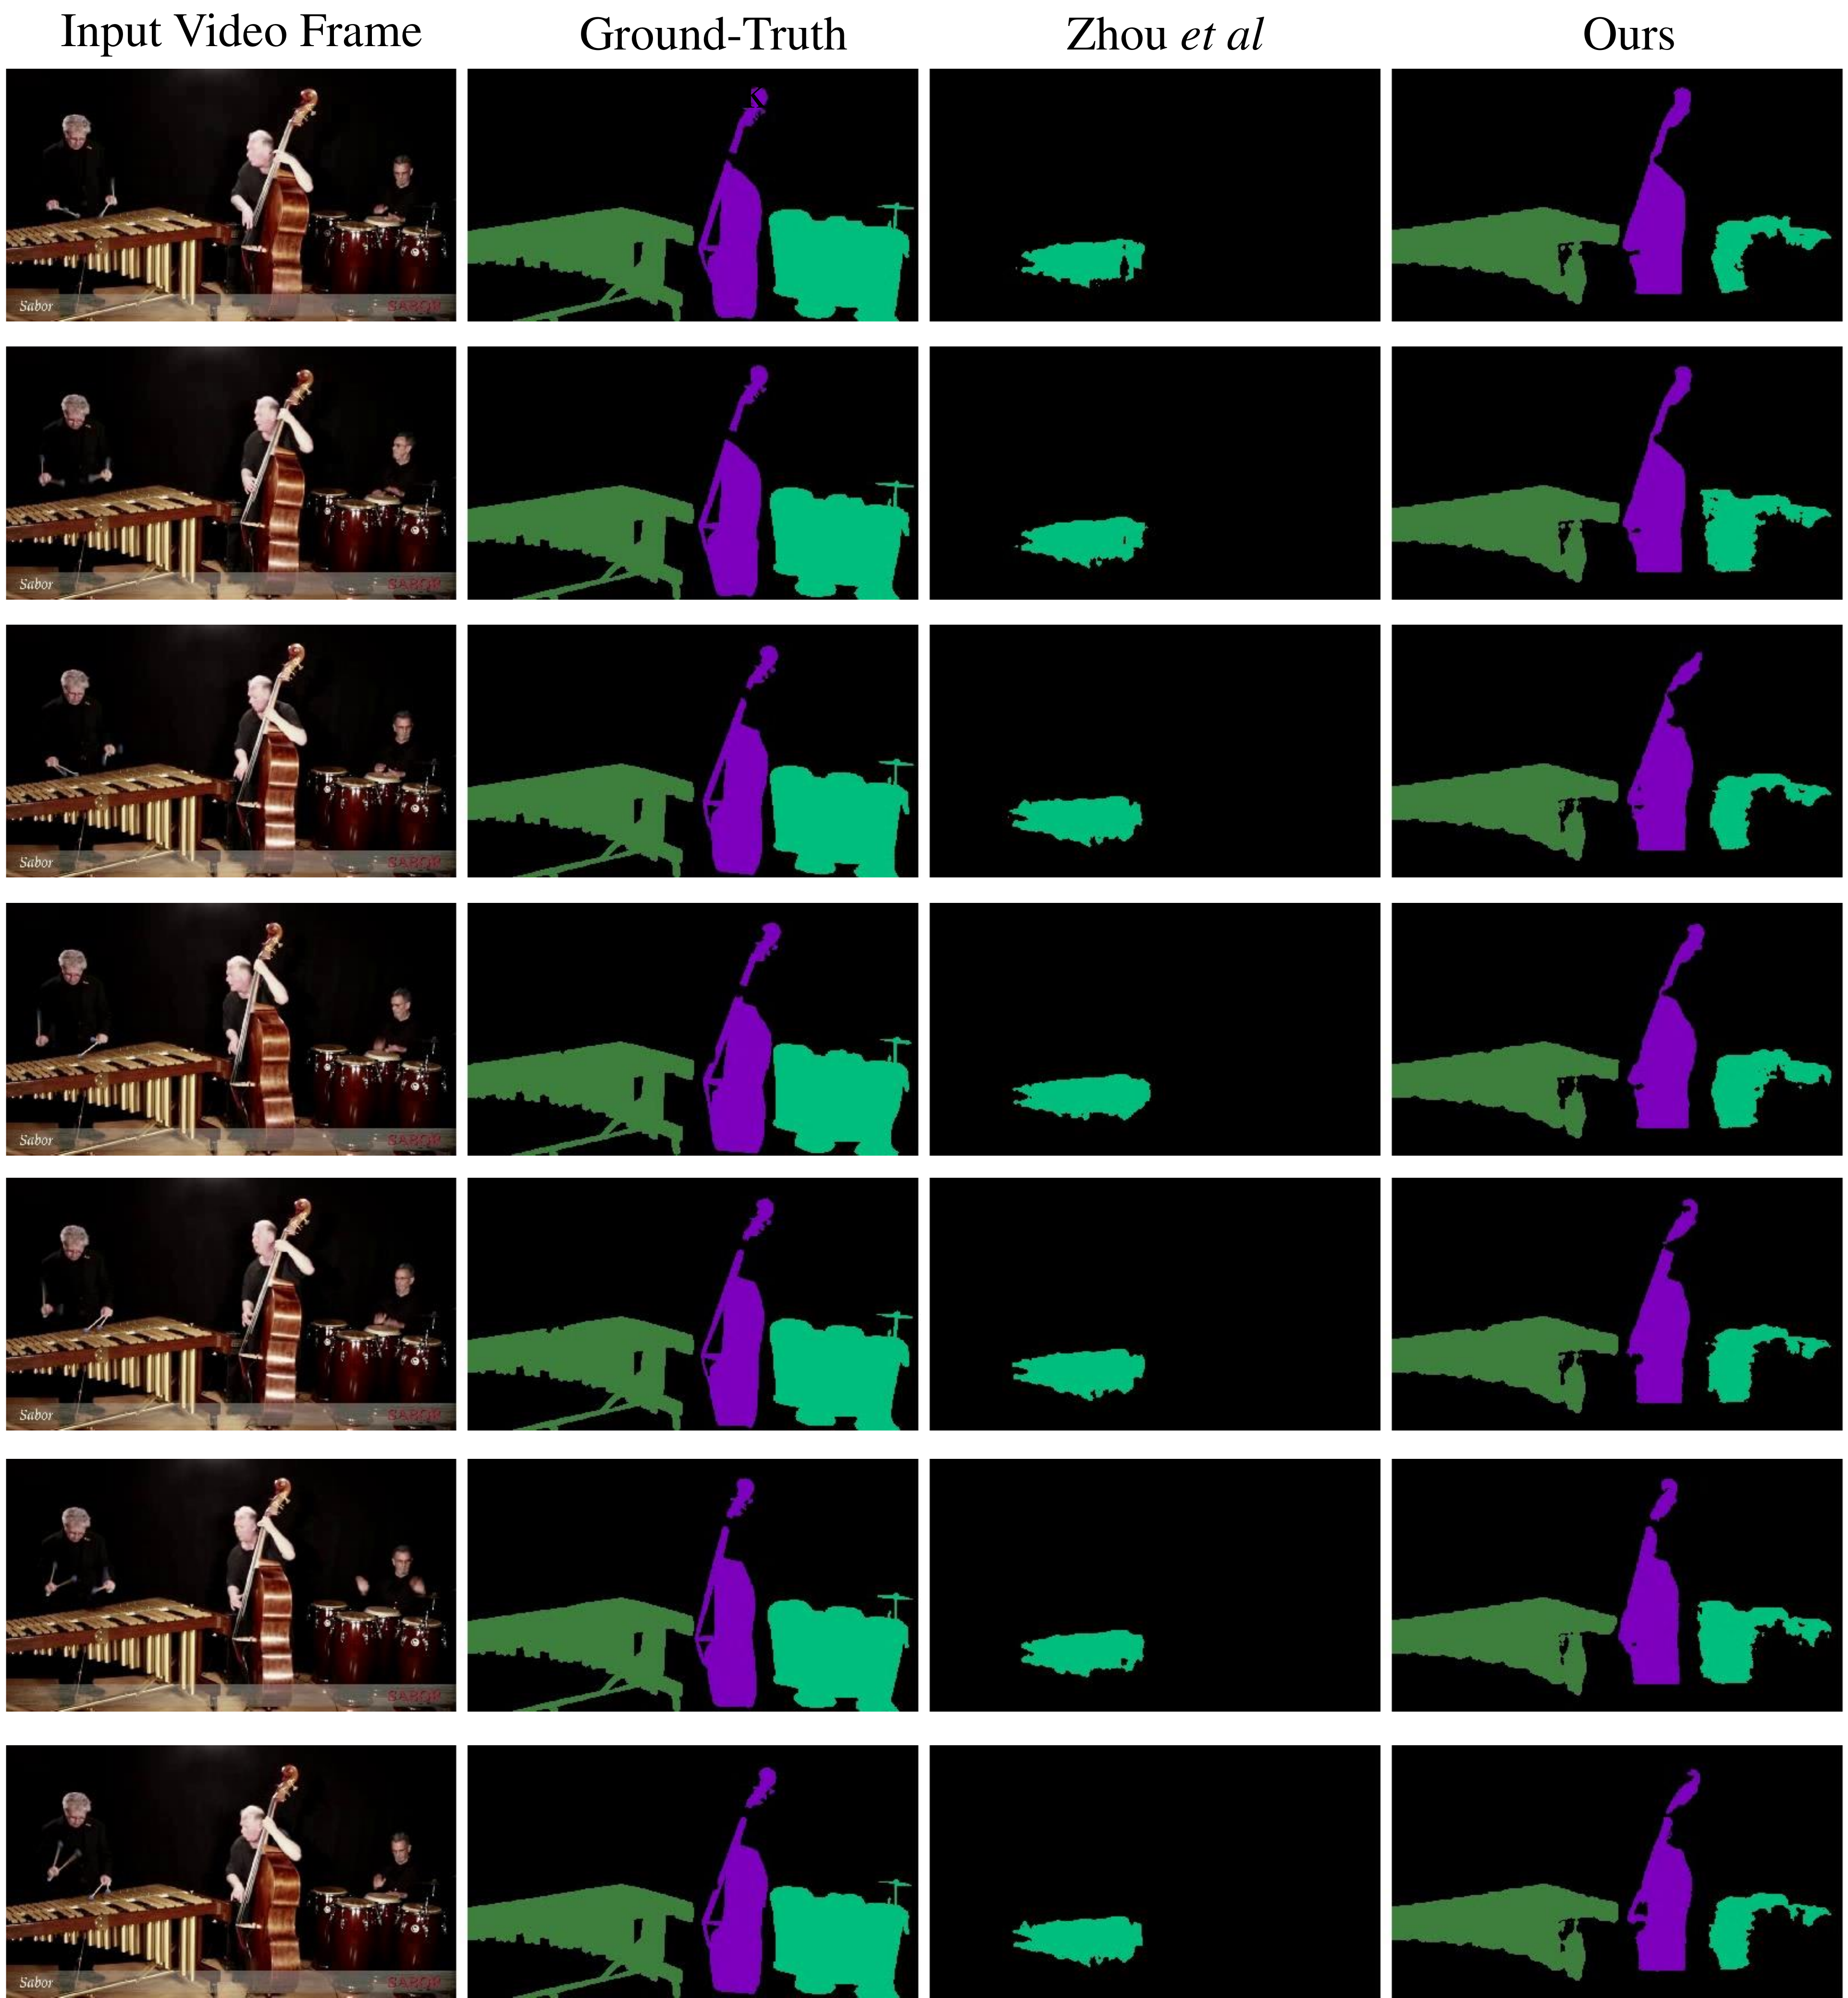}
    }
    \caption{Qualitative comparison to  Zhou \etal$\,$ \cite{zhou2023audio} on AVS-Semantic. Each color represents a semantic category. Our model excels in accurately segmenting \textbf{multiple sounding objects}, showcasing its proficiency in audio-guided segmentation. This success can be attributed to the effective utilization of a decomposed and discretized audio representation, which enables the model to capture and analyze the distinct acoustic features of each object, resulting in precise segmentation outcomes.}
    \label{fig:qualitative_2}
\end{figure*}

\begin{figure*}[t]
    \centering
    \scalebox{1}{
    \includegraphics[width=\linewidth]{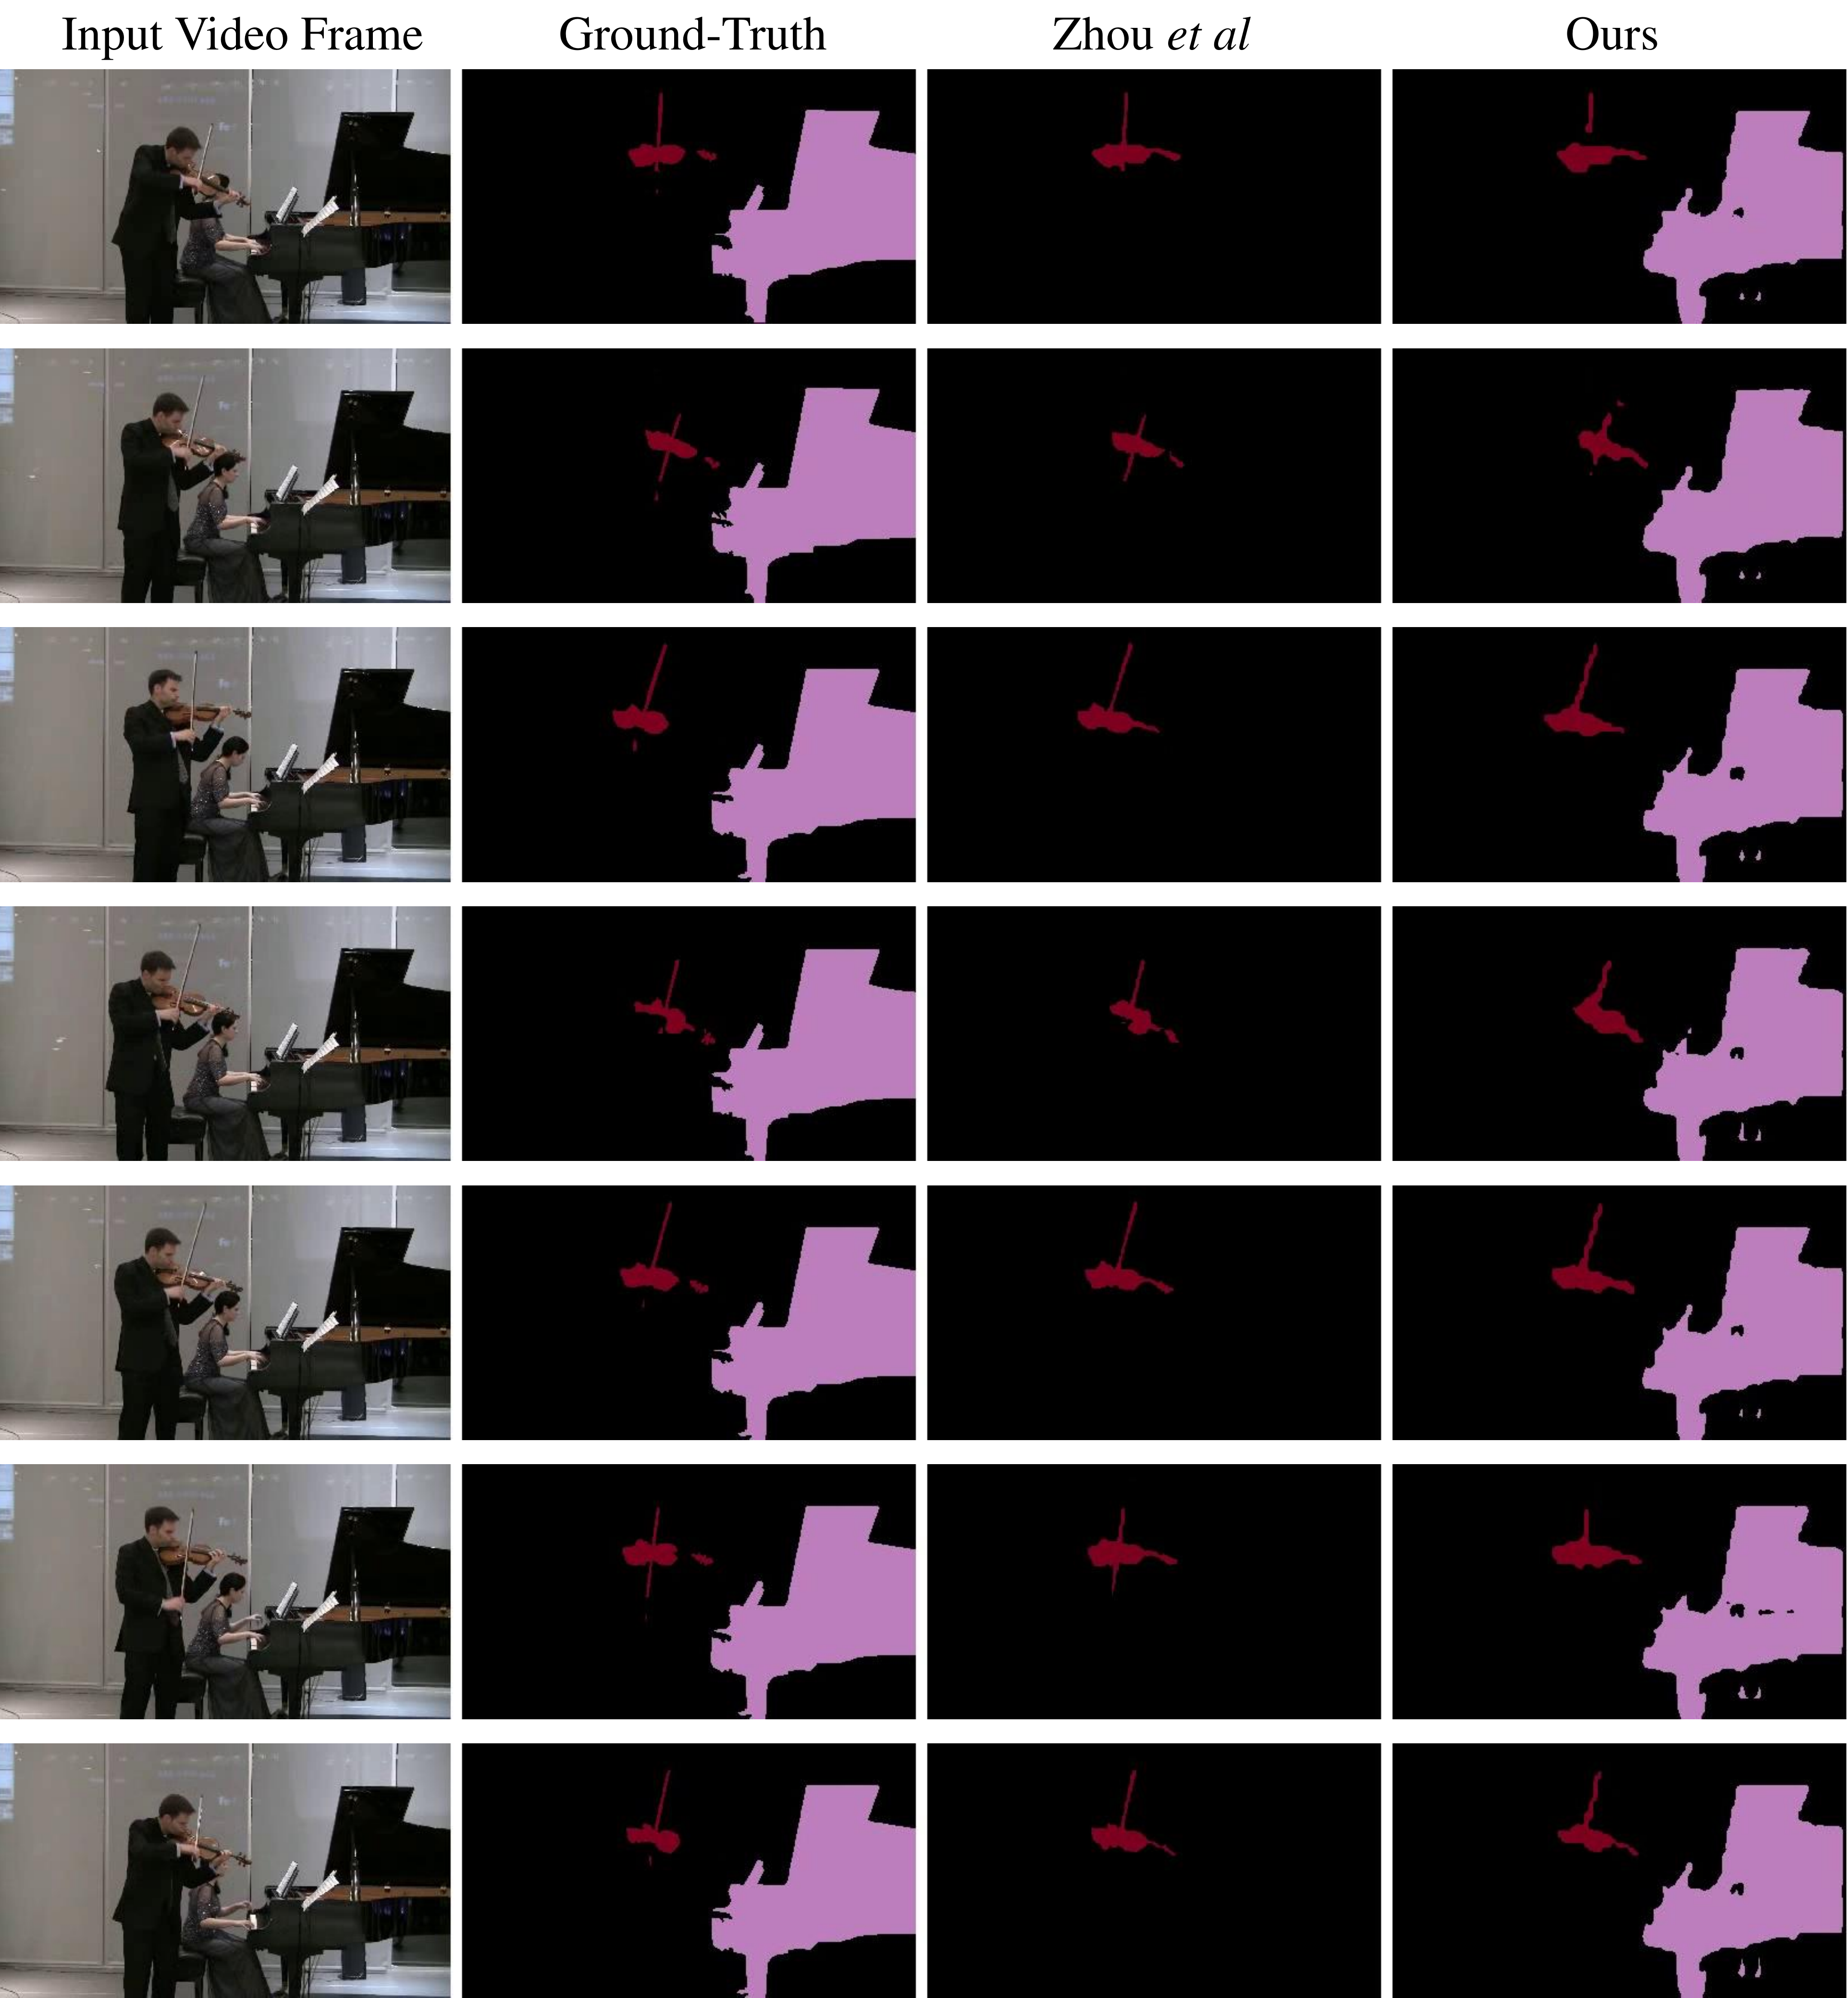}
    }
    \caption{Qualitative comparison to  Zhou \etal$\,$ \cite{zhou2023audio} on AVS-Semantic. Each color represents a semantic category. Our model excels in accurately segmenting \textbf{multiple sounding objects}, showcasing its proficiency in audio-guided segmentation. This success can be attributed to the effective utilization of a decomposed and discretized audio representation, which enables the model to capture and analyze the distinct acoustic features of each object, resulting in precise segmentation outcomes.}
    \label{fig:qualitative_3}
\end{figure*}

\begin{figure*}[t]
    \centering
    \scalebox{1}{
    \includegraphics[width=\linewidth]{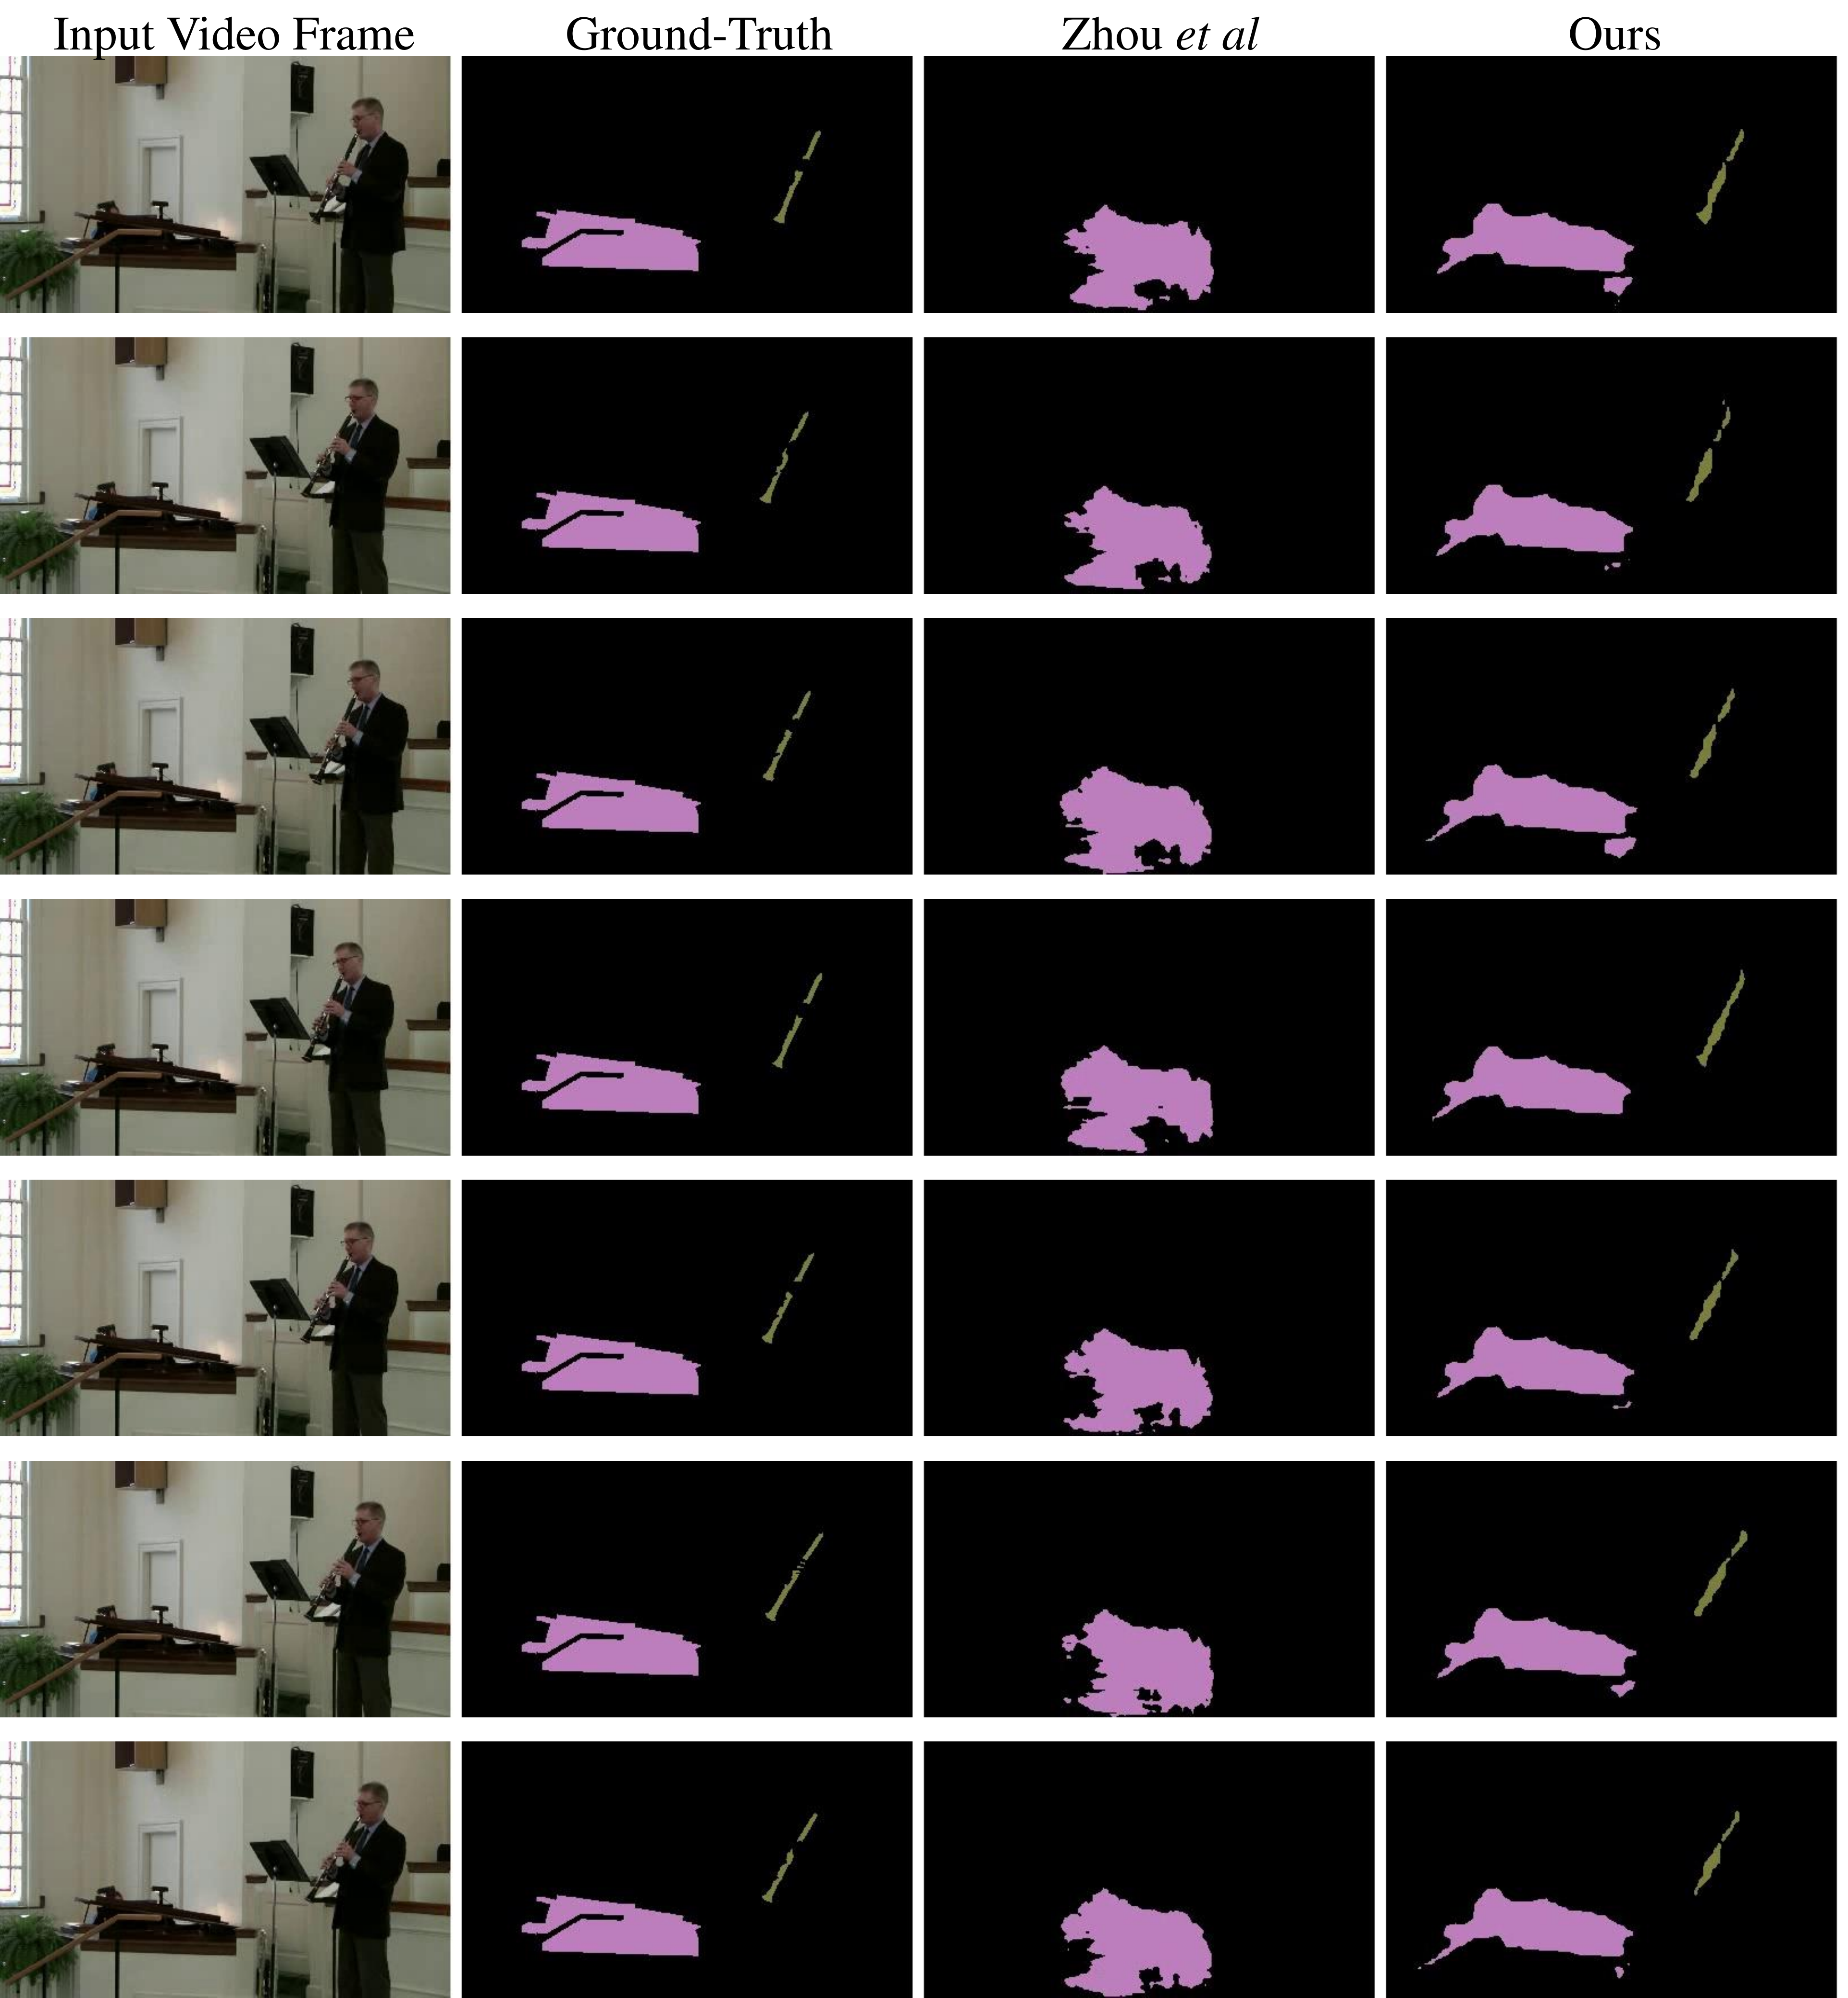}
    }
    \caption{Qualitative comparison to  Zhou \etal$\,$ \cite{zhou2023audio} on AVS-Semantic. Each color represents a semantic category. Our model demonstrates remarkable proficiency in accurately segmenting \textbf{tiny sounding objects}, owing to the implementation of a decomposed and discretized audio representation. By leveraging this technique, our model effectively captures the intricate acoustic details and nuances of these small-sized objects, resulting in precise and reliable segmentation outcomes. }
    \label{fig:qualitative_4}
\end{figure*}

% \begin{figure}[t]
%     \centering
%     \scalebox{1}{
%     \includegraphics[width=\linewidth]{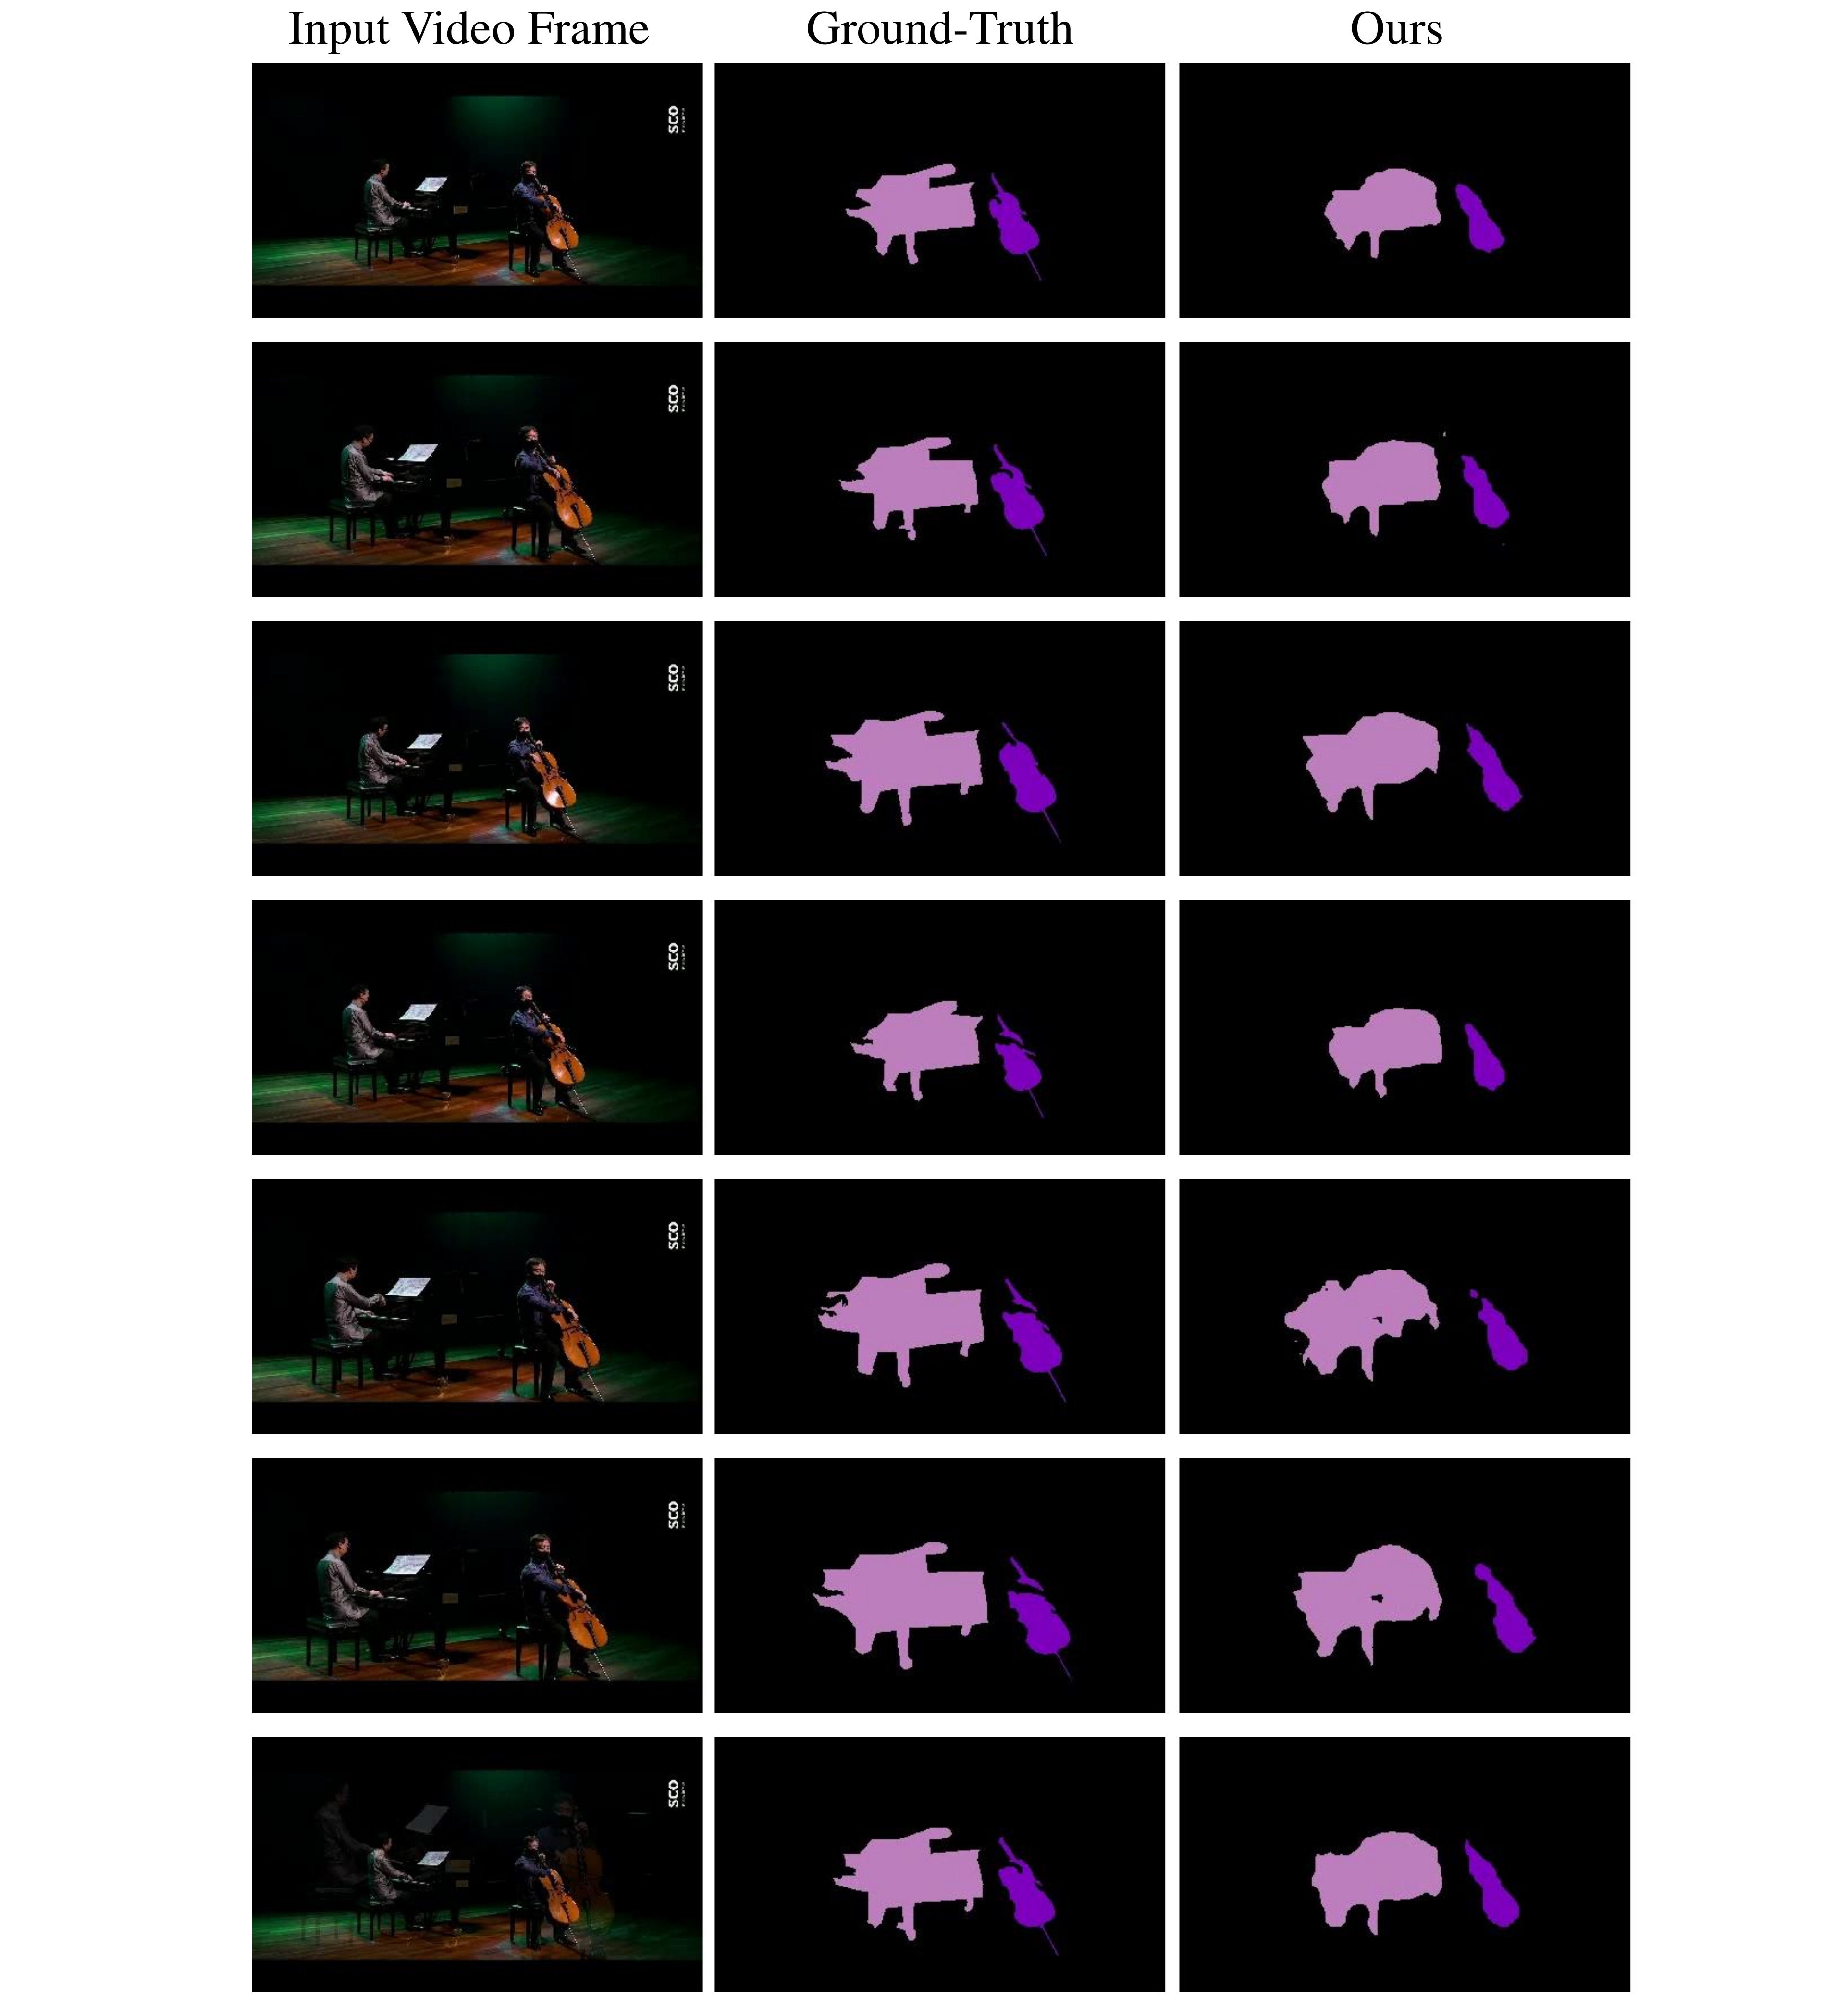}
%     }
%     \caption{Failure case. In this case, although our model can roughly distinguish the sounding objects, the boundary of the piano is not segmented well by our model.}
%     \label{fig:failure}
% \end{figure}

\section{More details about inference}
To tackle scenarios where queried content keeps changing, we perform per-frame inference. For each time $t$, we assign a class to the pixel at $[h, w]$ by
\begin{equation}
\arg\max_{C\in\{1,\cdots,K\}}\sum_{i=1}^NP_{i,t}[C]M_{i,t}[h,w],
\end{equation}
where $P_{i,t}[C]$ is the probability of class $C$.
Note that $\arg\max$ does not include the ``empty'' category ($\emptyset$) as AVS requires each output pixel to belong to one semantic category.
